# Supplementary material for: SoK: Technical Implementation and Human Impact of Internet Privacy Regulations
Source: arXiv:2312.15383 source file (2023-12-24)
Supplement: Supplementary file 1 [file 90-appendix.tex]

\section*{Appendix}
This is the appendix

    \subsubsection {Brazil}
    Brazil’s Lei Geral de Proteção de Dados (LGPD) became effective on August 1, 2021, and applies to controllers and processors of personal information, regardless of an entity’s location, when any of the following apply: (i) The processing is carried out within Brazil; (ii) The purpose of the processing is to offer or provide goods or services to individuals located within Brazil; or (iii) The personal data processed is collected in Brazil.

Under the LGPD, “Personal data” is defined as any information related to a natural person identified or identifiable.” (Article 5, I). The LGDP also delineates certain personal data as sensitive (and thus subject to specific processing conditions), including personal data concerning racial or ethnic origin, religious belief, political opinion, trade union or religious, philosophical or political organization membership, data concerning health or sex life, genetic or biometric data, when related to a natural person. (Article 5, II)

Under the LGPD, data subjects maintain the following data privacy rights, though the scope and condition for each may vary depending on both circumstances and local law: (a) right to access the data subject’s own personal data; (b) right to rectify/correct the data subject’s own personal data where inaccurate or incomplete; (c) right to erasure of personal data; (d) right to restrict data processing; (e) right to data portability; (f) right to object to the processing of personal data; (g) right to withdraw consent; (h) right to ask for data to be anonymized; (i) right to lodge a complaint before the ANPD; (j) right to obtain a copy when the legal basis for processing is consent or performance of a contract;(k) right to anonymize, block or delete unnecessary or excessive personal data, or data processed without compliance with the LGPD;(l) right to be informed about the public and private entities with whom the data has been shared; and (m) right to review decisions made solely on the basis of automated processing.

The LGPD imposes a variety of business obligations, including: (a) notice and transparency requirements, (b) legal basis for processing, (c) purpose limitations, (d) data minimization, (e) security requirements; (f) processor/service provider requirements; (g) prohibition on discrimination; (h) record keeping; (i) risk/impact assessments; (j) data breach notification; (k) data protection officer; and (l) international data transfer restrictions. 

    \subsubsection {Canada}
    Canada’s Personal Information and Electronic Documents Act (PIPEDA) became effective January 1, 2001 and applies to (i) the collection, use and disclosure of personal information by an organization in the course of its commercial activity in a province without substantially similar privacy legislation; (ii) the transfer of personal information across borders; (iii) federal works, undertakings or businesses (FWUBs); and (iv) the collection, use and disclosure of employee information in connection with FWUBs. The provinces of Alberta, British Columbia, and Quebec have enacted private sector privacy laws which apply to the collection, use, and disclosure of personal information within those provinces: AB PIPA, BC PIPA, and the Quebec Private Sector Act. Unlike PIPEDA, these statutes apply regardless of whether an activity is commercial in nature and apply to employee personal information.
    
Under the PIPEDA, “personal data” means information about an identifiable individual and thus offers broad interpretation. Information generally fits the definition of 'personal information' under PIPEDA where there is a reasonable possibility that an individual could be identified using the information, alone or in combination with other available information. “Sensitive data” is not defined under PIPEDA, AB PIPA, or BC PIPA, but PIPEDA provides that 'any information can be sensitive depending on the context' and thus subjects it to specific processing conditions

Under the PIPEDA, data subjects maintain the following data privacy rights, though the scope and condition for each may vary depending on both circumstances and local law: (a) right to access the data subject’s own personal data ; (b) right to rectify/correct the data subject’s own personal data where inaccurate or incomplete ; (c) right to erasure of personal data; (d) right to restrict data processing; and (e) right to object to the processing of personal data.

The PIPEDA imposes a variety of business obligations, including: (a) notice and transparency requirements, (b) legal basis for processing, (c) purpose limitations, (d) data minimization, (e) security requirements; (f) record keeping; (g) data breach notification; and (h) data protection officer.

\subsubsection{European Union Cookie Directive}
Directive 2009/136/EC, also colloquially known as the EU Cookie Directive, became effective in May 2011 and governs the processing of personal data and the protection of privacy in the electronic communications sector. The EU Cookie Directive is an amendment of Directive 2002/58/EC, which is often referred to as the “E-privacy Directive. “The EU Cookie Directive (and e-Privacy directive more broadly) applies to all countries within the EU, websites that are owned by EU companies, and international websites that cater to EU citizens. 
    
Under the EU cookie directive, Companies are required to obtain informed consent for storage or access of data on electronic devices. The directive’s requirement applies to all types of information on the terminal device; however the majority of legal and policy research and discourse has been on its implications for the usage of cookies (hence the its moniker). Specifically, Article 5.3 provides, “Member states shall ensure that the use of electronic communications networks to store information or to gain access to information stored in the terminal equipment of a subscriber or user is only allowed on condition that the subscriber or user concerned is provided with clear and comprehensive information in accordance with Directive 95/46/EC, inter alia about the purposes of the processing, and is offered the right to refuse such processing by the data controller. This shall not prevent any technical storage or access for the sole purpose of carrying out or facilitating the transmission of a communication over an electronic communications network, or as strictly necessary in order to provide an information society service explicitly requested by the subscriber or user.” In effect, the EU cookie directive requires companies to afford users both: (1). clear and comprehensive information about the purposes of processing and (2) the right to refuse such processing. 

\subsubsection{European Union General Data Protection Regulation (GDPR)}
    The European Union's General Data Protection Regulation (GDPR) became effective on May 25, 2018 and applies to data controllers and data processors that are: (1) established in the EU and process personal data in the context of activities of the EU establishment, regardless of whether the data processing takes place in the EU; (2) Not established in the EU and process personal data of EU data subjects in connection with offering goods or services in the EU (or otherwise monitoring the behavior of EU data subjects).

Under the GDPR, "Personal data" is defined as any information relating to an identified or identifiable natural person, where an "identifiable person" is one who can be identified, directly or indirectly, in particular by reference to an identifier such as a name, identification number, location data, online identifier or to one or more factors specific to the physical, physiological, genetic, mental, economic, cultural or social identity of that natural person (article 4 of the GDPR, article 2 of the Data Protection Act).

The GDPR also delineates certain personal data as “sensitive” (and thus subject to specific processing conditions), including: (i) racial or ethnic origin; (ii) political opinions; religious or philosophical beliefs; (iii) trade-union membership; (iv) genetic data; (v) biometric data processed solely to identify a human being; (vi) health-related data; (vii) sex life or sexual orientation. 

Under the GDPR, data subjects maintain the following data privacy rights, though the scope and condition for each may vary depending on both circumstances and local law: (a) right to access the data subject’s own personal data; (b) right to rectify/correct the data subject’s own personal data where inaccurate or incomplete; (c) right to erasure of personal data; (d) right to restrict data processing; (e) right to data portability; (f) right to object to the processing of personal data; and (g) right to withdraw consent.

The GDPR imposes a variety of business obligations, including: (a) notice and transparency requirements, (b) legal basis for processing, (c) purpose limitations, (d) data minimization, (e) security requirements; (f) privacy by design; (g) processor/service provider requirements; (h) prohibition on discrimination; (i) record keeping; (j) risk/impact assessments; (k) data breach notification; (l) registration with authorities; (m) data protection officer; and (l) international data transfer restrictions.

    \subsubsection{CCPA}
    The California Consumer Protection Act (CCPA) became effective on January 1, 2020 and applies to for profit entities that collect personal information from California residents and when any of the following thresholds apply: (i) At least 25 million in gross annual revenue; (ii) Buys, sells, or receives personal information about at least 50,000 California consumers, households or devices for commercial purposes; or (iii) Derives more than 50 percent of its annual revenue from the sale of personal information.
The CCPA defines “personal information" as “information that identifies, relates to, describes, is reasonably capable of being associated with, or could reasonably be linked, directly or indirectly, with a particular consumer or household. Personal information includes, but Is riot limited to, the following If It identifies, relates to, describes, is reasonably capable of being associated with, or could be reasonably linked, directly or indirectly, with a particular consumer or household” and further establishes eleven categories of personal information (including examples for each): identifiers, customer records information, characteristics of protected classifications under California or federal law, commercial information, biometric information, internet or other electronic network activity information, geolocation data, audio/electronic/visual/thermal/olfactory/or other similar information, professional or employment-related information, education information, and inferences. Section 1798.140.(o)

Under the CCPA, data subjects maintain the following data privacy rights, though the scope and condition for each may vary depending on both circumstances and local law: (a) right to access the data subject’s own personal data; (b) right to erasure of personal data; (c) right to opt-out of personal information sales; (d) right to nondiscrimination; and (e) right to data portability.

The CCPA imposes a variety of business obligations, including: (a) notice and transparency requirements, (b) purpose limitations, (c) security requirements; (d) processor/service provider requirements; (e) prohibition on discrimination; and (f) record keeping. 

    \subsubsection{CPRA}
    The California Privacy Rights Act (CPRA) amends the California Consumer Protection Act (CCPA) and soon becomes effective on January 1, 2023. The CPRA amends the CCPA’s application thresholds such that the combined legislations applies to for profit entities that collect personal information from California residents and when any of the following thresholds apply: (i) At least 25 million in gross annual revenue; (ii) Buys, sells, or shares personal information of 100,000 or more California residents or households; or (iii) Derives 50 percent or more of its annual revenue from selling or sharing California personal information.
    
The CPRA does not amend the CCPA’s definition of “personal information,” but the CPRA does introduce “sensitive personal information” as a subcategory of personal information subject to specific conditions, defining it as personal information that reveals: (i) A consumer’s social security, driver’s license, state identification card, or passport number; (ii) A consumer’s account log-in, financial account, debit card, or credit card number in combination with any required security or access code, password, or credentials allowing access to an account; (iii) A consumer’s precise geolocation; (iv) A consumer’s racial or ethnic origin, religious or philosophical beliefs, or union membership; (v) The contents of a consumer’s mail, email, and text messages unless the business is the intended recipient of the communication; (vi) A consumer’s genetic data.

Sensitive personal information under the CPRA also includes: (i) The processing of biometric information for the purpose of uniquely identifying a consumer; (ii) Personal information collected and analyzed concerning a consumer’s health; (iii) Personal information collected and analyzed concerning a consumer’s sex life or sexual orientation.

Under the CPRA, data subjects maintain the following data privacy rights, though the scope and condition for each may vary depending on both circumstances and local law: (a) right to access the data subject’s own personal data; (b) right to erasure of personal data; (c) right to opt-out of personal information sales; (d) right to nondiscrimination; and (e) right to data portability; (f) right to rectify/correct the data subject’s own personal data where inaccurate or incomplete; (g) right to opt out of sharing for cross-context behavior advertising; (h) right to restrict data processing; and (i) right to opt-out of the use of automated decision-making.

The CPRA imposes a variety of business obligations, including: (a) notice and transparency requirements, (b) purpose limitations, (c) data minimization, (d) security requirements; (e) processor/service provider requirements; (f) prohibition on discrimination; and (g) risk/impact assessments. 

    \subsubsection{Singapore}
    Singapore’s Personal Data Protection Act (PDPA) became effective on January 2, 2013.Singapore’s Personal Data Protection (Amendment) Act (PDPAA) became effective on February 1, 2021. Both (which we collectively refer to as PDPA) generally apply to all private organizations in respect of the personal data of individuals that they collect, use, and/or disclose, including organizations with no physical presence in Singapore, if these organizations collect, use, or disclose data within Singapore.

"Personal data" under the PDPA refers to all "data, whether true or not, about an individual who can be identified from that data, or from that data and other information to which the organization has or is likely to have access". There is no definition of sensitive personal data under the PDPA, but non-binding guidance from Singapore’s Personal Data Protection Commission indicates that sensitivity of data is a factor for consideration in implementing policies and procedures to ensure appropriate levels of security for personal data.

Under the PDPA, data subjects maintain the following data privacy rights, though the scope and condition for each may vary depending on both circumstances and local law: (i) right to access the data subject’s own personal data; (ii) right to rectify/correct the data subject’s own personal data where inaccurate or incomplete; (iii) right to withdraw consent. 

The PDPA imposes a variety of business obligations, including: (a) notice and transparency requirements, (b) legal basis for processing, (c) purpose limitations, (d) data minimization, (e) security requirements; (f) processor/service provider requirements; (g) record keeping; (h) data breach notification; (i) registration with authorities; (j) data protection officer; and (k) international data transfer restrictions. 

    \subsubsection {South Korea}
    South Korea’s Personal Information Protection Act (PIPA) became effective on September 30, 2011 and applies to (a) personal information controllers, which means a public institution, legal person, organization, individual, etc. that processes personal information directly or indirectly to operate the personal information files as part of its activities, and (b) personal information handlers, who are persons who process the personal information under the command and supervision of a personal information controller, such as an officer or employee, temporary agency worker and part-time worker

Under the PIPA, “personal information” means information relating to a living individual that constitutes any of the following: (a) Information that identifies a particular individual by his/her full name, resident registration number, image, etc.; (b) Information which, even if by itself does not identify a particular individual, may be easily combined with other information to identify a particular individual (in this case, whether or not there is ease of combination shall be determined by reasonably considering the time, cost, technology, etc. used to identify the individual such as likelihood that the other information can be procured); or (c) Information under items (a) or (b) above that is pseudonymized in accordance with the relevant provisions and thereby becomes incapable of identifying a particular individual without the use or combination of information for restoration to the original state (referred to as “pseudonymized information”).

Under the PIPA, “sensitive information” is defined as personal information concerning an individual’s ideology, faith, labor union membership, political views or membership in a political party, health or medical treatment information, sexual orientation, genetic information, criminal records and biometric data for the purpose of uniquely identifying a natural person and race/ethnic information. 

Under the PIPA, data subjects maintain the following data privacy rights, though the scope and condition for each may vary depending on both circumstances and local law: (a) right to access the data subject’s own personal data; (b) right to rectify/correct the data subject’s own personal data where inaccurate or incomplete; (c) right to erasure of personal data; (d) right to object to the processing of personal data; and (e) right to withdraw consent.

The PIPA imposes a variety of business obligations, including: (a) notice and transparency requirements, (b) legal basis for processing, (c) purpose limitations, (d) data minimization, (e) security requirements; (f) processor/service provider requirements; (g) record keeping; (h) risk/impact assessments; (i) data breach notification; (j) registration with authorities; (k) data protection officer; and (l) international data transfer restrictions.

    \subsubsection {United States COPPA}
    The United States Congress established the Children’s Online Privacy Protection Act (COPPA) in 1998. COPPA prohibits unfair or deceptive acts or practices in connection with the collection, use, and/or disclosure of personal information from and about children on the Internet and requires the Federal Trade Commission (FTC) to issue and enforce regulations concerning children’s online privacy. The FTC’s original COPPA Rule became effective on April 21, 2000. The FTC published an amended Rule on January 17, 2013. The amended Rule took effect on July 1, 2013. Hereinafter, we refer to COPPA and the COPPA Rule as COPPA.

COPPA applies to (a) operators of commercial websites and online services (including mobile apps and IoT devices) directed to children under 13 that collect, use, or disclose personal information from children; (b) operators of general audience websites or online services with actual knowledge that they are collecting, using, or disclosing personal information from children under 13; and (c) websites or online services that have actual knowledge that they are collecting personal information directly from users of another website or online service directed to children.

Under COPPA, personal information means individually identifiable information about an individual collected online, including: First and last name; A home or other physical address including street name and name of a city or town; Online contact information; A screen or user name that functions as online contact information; A telephone number; A Social Security number; A persistent identifier that can be used to recognize a user over time and across different websites or online services; A photograph, video, or audio file, where such file contains a child’s image or voice; Geolocation information sufficient to identify street name and name of a city or town; or Information concerning the child or the parents of that child that the operator collects online from the child and combines with an identifier described above. 16 CFR 312.2 “Personal information”

Operators subject to COPPA must: (1.) Post a clear and comprehensive online privacy policy describing their information practices for personal information collected online from children; (2.) Provide direct notice to parents and obtain verifiable parental consent, with limited exceptions, before collecting personal information online from children; (3.) Give parents the choice of consenting to the operator’s collection and internal use of a child’s information, but prohibiting the operator from disclosing that information to third parties (unless disclosure is integral to the site or service, in which case, this must be made clear to parents); (4.) Provide parents access to their child's personal information to review and/or have the information deleted; (5.) Give parents the opportunity to prevent further use or online collection of a child's personal information; (6.) Maintain the confidentiality, security, and integrity of information they collect from children, including by taking reasonable steps to release such information only to parties capable of maintaining its confidentiality and security; (7.) Retain personal information collected online from a child for only as long as is necessary to fulfill the purpose for which it was collected and delete the information using reasonable measures to protect against its unauthorized access or use; and (8.) Not condition a child’s participation in an online activity on the child providing more information than is reasonably necessary to participate in that activity.
